# Supplementary material for: Forbidden Backscattering and Resistance Dip in the Quantum Limit as a Signature for Topological Insulators
Source: arXiv:1801.03617 source file (2018-07-21)
Supplement: Supplementary file 1 [file TI-QL-supp-20180424.pdf]

# Supplemental Material for “Forbidden Backscattering and Resistance Dip in the Quantum Limit as a Signature for Topological Insulators”

Yiyuan Chen,<sup>1,2</sup> Hai-Zhou Lu,<sup>1,2,\*</sup> and X. C. Xie<sup>3,4</sup>

<sup>1</sup>*Shenzhen Institute for Quantum Science and Technology and Department of Physics,  
Southern University of Science and Technology, Shenzhen 518055, China*

<sup>2</sup>*Shenzhen Key Laboratory of Quantum Science and Engineering, Shenzhen 518055, China*

<sup>3</sup>*International Center for Quantum Materials, School of Physics, Peking University, Beijing 100871, China*

<sup>4</sup>*Collaborative Innovation Center of Quantum Matter, Beijing 100871, China*

(Dated: May 7, 2018)

In this Supplemental Material, we present the calculations for those in the list of contents.

## CONTENTS

|                                                                             |    |
|-----------------------------------------------------------------------------|----|
| S1. Landau bands                                                            | S1 |
| S2. Calculation of conductivity                                             | S2 |
| A. Transport time                                                           | S2 |
| 1. Transport time for Gaussian potential                                    | S3 |
| 2. Transport time for Screened Coulomb potential                            | S3 |
| B. Transport time for Spin-orbit Scattering                                 | S3 |
| 1. Transport time for diagonal spin-orbit scattering                        | S4 |
| 2. Transport time for off-diagonal Spin-orbit Scattering                    | S4 |
| 3. Total transport time and the resistivity                                 | S5 |
| 4. Definition of magnetoresistance                                          | S6 |
| C. Scattering matrix elements                                               | S6 |
| D. Numerical scheme for $\Lambda$                                           | S7 |
| S3. $B_c$ for the $\text{Bi}_2\text{Se}_3$ family                           | S7 |
| S4. Comparison with the experiment on $\text{Pb}_{1-x}\text{Sn}_x\text{Se}$ | S7 |
| S5. Resistivity in the presence of Gaussian scattering potential            | S8 |
| References                                                                  | S8 |

## S1. LANDAU BANDS

In a magnetic field along the  $z$  direction, using Landau gauge  $\mathbf{A} = (-By, 0, 0)$  and the ladder operator

$$k_- = \frac{\sqrt{2}}{\ell_B} a_-, \quad k_+ = \frac{\sqrt{2}}{\ell_B} a_+, \quad (\text{S1})$$

where  $\ell_B = \sqrt{\hbar/eB}$ . With the trial wave function  $(|\nu - 1\rangle, |\nu\rangle, |\nu - 1\rangle, |\nu\rangle)^T$ , the original Hamiltonian becomes

$$H = C_0 + C_z k_z^2 + \begin{bmatrix} m_1 & 0 & iV_n k_z & -i\frac{\sqrt{2\nu}V_\perp}{\ell_B} \\ 0 & m_2 & i\frac{\sqrt{2\nu}V_\perp}{\ell_B} & iV_n k_z \\ -iV_n k_z & -i\frac{\sqrt{2\nu}V_\perp}{\ell_B} & m_3 & 0 \\ i\frac{\sqrt{2\nu}V_\perp}{\ell_B} & -iV_n k_z & 0 & m_4 \end{bmatrix},$$

where

$$\begin{aligned} m_1 &= \frac{2(C_\perp + M_\perp)}{\ell_B^2}(\nu - \frac{1}{2}) + M_z k_z^2 + g_1 B_z + M_0, \\ m_2 &= \frac{2(C_\perp + M_\perp)}{\ell_B^2}(\nu + \frac{1}{2}) + M_z k_z^2 - g_1 B_z + M_0, \\ m_3 &= \frac{2(C_\perp - M_\perp)}{\ell_B^2}(\nu - \frac{1}{2}) - M_z k_z^2 + g_2 B_z - M_0, \\ m_4 &= \frac{2(C_\perp - M_\perp)}{\ell_B^2}(\nu + \frac{1}{2}) - M_z k_z^2 - g_2 B_z - M_0, \end{aligned} \quad (\text{S2})$$

and  $g_z^v = 2g_1/\mu_B$ ,  $g_z^c = 2g_2/\mu_B$ .

In the quantum limit, only the  $\nu = 0$  band is occupied by the electrons, so we only focus on  $\nu = 0$ , the trial wave function becomes  $(0, |0\rangle, 0, |0\rangle)^T$ , the Hamiltonian becomes

$$H = C_0 + C_z k_z^2 + \begin{bmatrix} m_2 & iV_n k_z \\ -iV_n k_z & m_4 \end{bmatrix}, \quad (\text{S3})$$

where

$$\begin{aligned} m_2 &= \frac{(C_\perp + M_\perp)}{\ell_B^2} + M_z k_z^2 - g_1 B_z + M_0, \\ m_4 &= \frac{(C_\perp - M_\perp)}{\ell_B^2} - M_z k_z^2 - g_2 B_z - M_0. \end{aligned} \quad (\text{S4})$$

Its eigenvalues are

$$E_{0\pm} = C_0 + C_z k_z^2 - \frac{g_+ B_z}{2} + \frac{C_\perp}{\ell_B^2} \pm \sqrt{m^2 + V_n^2 k_z^2}, \quad (\text{S5})$$

\* Corresponding author. luhz@sustc.edu.cn

and the eigenvectors are

$$\begin{aligned}
 |0, +, k_x, k_z\rangle &= D_+ \begin{bmatrix} 0 \\ -iV_n k_z \\ 0 \\ m - \sqrt{m^2 + V_n^2 k_z^2} \end{bmatrix} |k_x, k_z, 0\rangle, \\
 |0, -, k_x, k_z\rangle &= D_- \begin{bmatrix} 0 \\ -iV_n k_z \\ 0 \\ m + \sqrt{m^2 + V_n^2 k_z^2} \end{bmatrix} |k_x, k_z, 0\rangle.
 \end{aligned}
 \tag{S6}$$

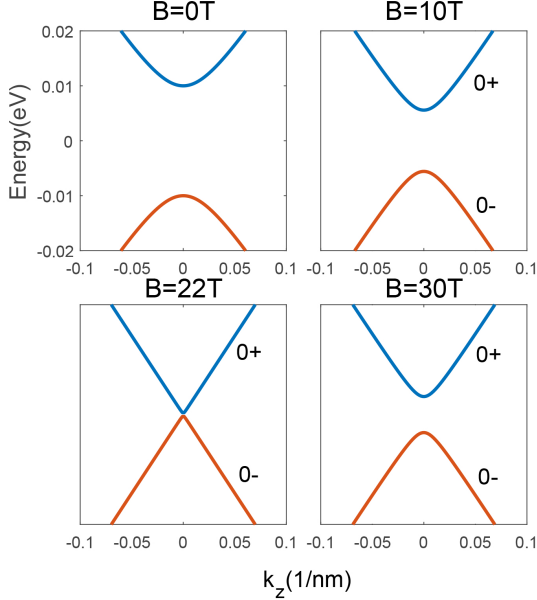

FIG. S1. The energies of the lowest Landau bands 0+ and 0- as functions of  $k_z$  at different magnetic fields. There is a band crossing at a critical magnetic field. The model parameters are  $M_0 = -0.010\text{eV}$ ,  $M_\perp = 13.50\text{eV}\cdot\text{\AA}^2$ ,  $M_z = 0$ ,  $-g_z^v = g_z^c = 7.5$ . We suppress the  $C_k$  term for simplicity.

## S2. CALCULATION OF CONDUCTIVITY

Along the  $z$  direction, the semiclassical Drude conductivity of the 0+ band can be found from the formula [1]

$$\sigma_{zz} = \frac{e^2 \hbar}{2\pi V} \sum_{k_z, k_x} \tilde{v}_{0+}^z G_{0+}^R v_{0+}^z G_{0+}^A, \tag{S7}$$

where  $-e$  is the electron charge,  $V = L_x L_y L_z$  is the volume with  $L_x$  the length along the  $x$  direction and so on,  $v_0^z = \partial E_{0+} / \hbar \partial k_z$  is the velocity along the  $z$  direction for a state with wave vector  $k_z$  in the  $\nu = 0$  band, and  $\tilde{v}_{0+}^z$  differs from  $v_{0+}^z$  up to a vertex correction from the disorder scattering [2].  $G_{0+}^{R/A} = 1/(E_F - E_{0+} \pm i\hbar/2\tau^{0+})$  is the retarded/advanced Green's function, with  $\tau^{0+}$  the lifetime of a state in the 0+ band. Usually, in the diffusive regime,

one can replace  $G_{0+}^R G_{0+}^A$  by  $\frac{2\pi}{\hbar} \tau^{0+} \delta(E_F - E_{0+})$ . However, in one dimension, to correct the van Hove singularity at the band edge, we introduce an extra correction factor  $\Lambda$ , so that  $G_{0+}^R G_{0+}^A = (2\pi/\hbar) \Lambda \tau^{0+} \delta(E_F - E_{0+})$ .  $\Lambda \rightarrow 1$  (0) if the Fermi energy is far away from (approaching) the band edge [3, 4]. Also, the vertex correction of  $v_{0+}^z$  to  $\tilde{v}_{0+}^z$  is equivalent to correct the lifetime  $\tau^{0+}$  to the transport time  $\tau_{\text{tr}}^{0+}$  [2]. The delta function

$$\delta(E_F - E_{0+}) = \frac{\delta(k_z - k_F)}{\hbar v_F} + \frac{\delta(k_z + k_F)}{\hbar v_F}, \tag{S8}$$

where  $v_F$  is the absolute value of the Fermi velocity of the 0+ band at the Fermi wave vectors  $\pm k_F$ . With the above calculations, the conductivity becomes

$$\sigma_{zz} = \frac{e^2}{h} \frac{\hbar v_F}{L_x L_y} \Lambda \sum_{k_x} \left( \frac{\tau_{k_F}^+}{\hbar} + \frac{\tau_{k_F}^-}{\hbar} \right), \tag{S9}$$

where  $\tau_{k_F}^\pm$  are the transport times at  $\pm k_F$ . The summation over  $k_x$  is limited by the Landau degeneracy, so

$$\sigma_{zz} = \frac{e^2}{h} \frac{\hbar v_F^0}{2\pi L_y} \Lambda \int_{-L_y/2\ell_B^2}^{L_y/2\ell_B^2} dk_x \left( \frac{\tau_{k_F}^+}{\hbar} + \frac{\tau_{k_F}^-}{\hbar} \right). \tag{S10}$$

It turns out that  $\tau_{k_F}^\pm$  are not functions of  $k_x$ , then

$$\sigma_{zz} = \frac{e^2}{h} \frac{\hbar v_F \Lambda}{2\pi \ell_B^2} \left( \frac{\tau_{k_F}^+}{\hbar} + \frac{\tau_{k_F}^-}{\hbar} \right). \tag{S11}$$

Using the transport times in Eq. (S21), for the Gaussian impurity scattering potential, Eq. (S11) becomes

$$\sigma_{zz} = \frac{e^2}{h} \frac{(\hbar v_F)^2 (2d^2 + \ell_B^2)}{V_{\text{imp}} \ell_B^2 I_S} e^{4d^2 k_F^2}. \tag{S12}$$

Using the transport time in Eq. (S28), for the screened Coulomb impurity scattering potential in the strong-field limit, Eq. (S11) becomes

$$\sigma_{zz} = \frac{e^2}{h} \frac{\hbar v_F^0 \Lambda \varepsilon}{\pi^2 n_{\text{imp}} e^2 \ell_B^4 I_S}. \tag{S13}$$

In Sec. S2D, we provide the scheme how  $\Lambda$  is calculated.

### A. Transport time

For the scattering among the states on the Fermi surface of the 0+ Landau band, the transport times can be found as

$$\begin{aligned}
 \frac{\hbar}{\tau_{k_F}^\pm} &= 2\pi \sum_{k'_x, k'_z} \langle |U_{0,0}^{\pm k_F, k'_z}|^2 \rangle \Lambda \delta(E_F - E_{0+}) \\
 &\quad \times \left[ 1 \mp \frac{v_{0+}^z(k'_z)}{v_F} \right],
 \end{aligned} \tag{S14}$$

where  $U_{0,0}^{\pm k_F, k'_z}$  represents the scattering matrix elements and  $\langle \dots \rangle$  means the impurity average. Considering there

are only two states on the Fermi surface with  $\pm k_F$ , i.e.,  $\delta(E_F - E_{0+}) = [\delta(k'_z - k_F) + \delta(k'_z + k_F)]/\hbar v_F$

$$\frac{\hbar}{\tau_{k_F}^{\pm}} = 4\pi \sum_{k'_x, k'_z} \langle |U_{0,0}^{k_z \pm k_F, k'_z}|^2 \rangle \frac{\Lambda \delta(k'_z \pm k_F)}{\hbar v_F}. \quad (\text{S15})$$

Using Eq. (S57) for the scattering matrix elements  $\langle |U_{0,0}^{k_z, k'_z}|^2 \rangle$ ,

$$\frac{\hbar}{\tau_{k_F}^{\pm}} = 2 \sum_{k'_x, k'_z} \int \frac{d^3 \mathbf{q}}{L_x L_z} \langle U^2(\mathbf{q}) \rangle e^{-q_{\perp}^2 \ell_B^2 / 2} \delta(q_x + k'_x - k_x) \times \delta(q_z + k'_z - k_z) \frac{\Lambda \delta(k'_z \pm k_F)}{\hbar v_F} \cos^2 \frac{\theta - \theta'}{2}, \quad (\text{S16})$$

where  $q_{\perp}^2 = q_x^2 + q_y^2$ . Changing the summations over  $k'_x, k'_z$  to integrals, Eq. (S16) can be simplified as

$$\frac{\hbar}{\tau_{k_F}^{\pm}} = 2 \frac{\Lambda I_S}{\hbar v_F} \int \frac{dq_x dq_y}{(2\pi)^2} \langle U^2(q_x, q_y, 2k_F) \rangle e^{-q_{\perp}^2 \ell_B^2 / 2}, \quad (\text{S17})$$

where  $I_S = \cos^2 \theta|_{k_F}$ .

### 1. Transport time for Gaussian potential

The transport time depends on the scattering potential of the impurities in materials. One of the convenient choices is the random Gaussian potential

$$U(\mathbf{r}) = \sum_i \frac{u_i}{(d\sqrt{2\pi})^3} e^{-|\mathbf{r} - \mathbf{R}_i|^2 / 2d^2}, \quad (\text{S18})$$

where  $u_i$  measures the scattering strength of a randomly distributed impurity at  $\mathbf{R}_i$ , and  $d$  is a parameter that determines the range of the scattering potential. Its Fourier transform is

$$U(\mathbf{q}) = \sum_i u_i e^{-q^2 d^2 / 2}. \quad (\text{S19})$$

Put it into Eq. (S17)

$$\frac{\hbar}{\tau_{k_F}^{\pm}} = 2 \frac{V_{\text{imp}} \Lambda I_S}{\hbar v_F e^{4d^2 k_F^2}} \int \frac{dq_x dq_y}{(2\pi)^2} e^{-q_{\perp}^2 (d^2 + \ell_B^2 / 2)}, \quad (\text{S20})$$

where  $V_{\text{imp}} \equiv \sum_i u_i^2 / V$ . Performing the integral in polar coordinates and we finally obtain

$$\frac{\hbar}{\tau_{k_F}^{\pm}} = I_S \frac{V_{\text{imp}}}{\hbar v_F} \frac{\Lambda e^{-4d^2 k_F^2}}{2\pi(d^2 + \ell_B^2 / 2)}. \quad (\text{S21})$$

### 2. Transport time for Screened Coulomb potential

Another choice of scattering potential is the Screened Coulomb potential [5]

$$U(\mathbf{r}) = \sum_i \frac{e^2}{4\pi\epsilon|\mathbf{r} - \mathbf{R}_i|} e^{-\kappa|\mathbf{r} - \mathbf{R}_i|}, \quad (\text{S22})$$

where  $\epsilon$  is the dielectric constant and  $1/\kappa$  is the screening length. The screened Coulomb potential is justified because excess silver atoms form clusters doping the rest of the material[5]. This potential is different from the ionic potential under the Thomas-Fermi approximation [6]. Following the standard random phase approximation [5, 7],

$$\kappa^2 = -\frac{e^2}{\epsilon} \frac{1}{2\pi\ell_B^2} \frac{1}{\beta} \times \sum_m \int_{-\infty}^{+\infty} \frac{dk_z}{2\pi} \frac{1}{(iw_m + E_F - E_{0+})^2}, \quad (\text{S23})$$

where  $\beta = 1/k_B T$ ,  $w_m = (2m + 1)\pi/\beta$  are the Matsubara frequencies of fermions. After summing over the Matsubara frequencies, we have

$$\frac{1}{\beta} \sum_m \frac{1}{(iw_m + E_F - E_{0+})^2} = \frac{\partial n_F(E_F - E_{0+})}{\partial(E_F - E_{0+})} \quad (\text{S24})$$

Substituting this into Eq. (S23), we have

$$\kappa^2 = \frac{e^2 \Lambda}{2\pi^2 \ell_B^2 \epsilon \hbar v_F}, \quad (\text{S25})$$

The Fourier transform is given by

$$U(\mathbf{q}) = \frac{e^2}{\epsilon(q^2 + \kappa^2)}. \quad (\text{S26})$$

Put it into Eq. (S17), and considering  $\ell_B^2 \kappa^2 \ll 1$  in strong magnetic fields, we have

$$\frac{\hbar}{\tau_{k_F}^{\pm}} = I_S n_{\text{imp}} \frac{\Lambda}{\hbar v_F^0} \frac{e^4}{\epsilon^2} \frac{1}{2\pi\kappa^2}. \quad (\text{S27})$$

By using Eq. (S25), we arrive at the transport time of the 0+ band in strong magnetic fields

$$\frac{\hbar}{\tau_{k_F}^{\pm}} = I_S \frac{\pi n_{\text{imp}} e^2 \ell_B^2}{\epsilon}. \quad (\text{S28})$$

## B. Transport time for Spin-orbit Scattering

For heavy-element impurities we consider spin-orbit scattering with the potential [8, 9]

$$U = \sum_i \nabla u(\mathbf{r} - \mathbf{R}_i) \times \mathbf{k} \cdot \mathbf{s} = \mathbf{U}^{\text{soc}} \cdot \mathbf{s}. \quad (\text{S29})$$

Our model is a  $4 \times 4$  Hamiltonian. According to the spin configuration of our basis ( $|\uparrow_1\rangle, |\downarrow_2\rangle, |\uparrow_3\rangle, |\downarrow_4\rangle$ ), the spin-orbit coupling can induce the scattering within 1 and 2 or 3 and 4 (diagonal) and those couple 1 and 2 to 3 and 4 (off-diagonal).

### 1. Transport time for diagonal spin-orbit scattering

First, we consider the diagonal spin-orbit scattering. The potential can be written in a matrix form

$$U = I_{2 \times 2} \otimes \begin{bmatrix} \mathbf{U}_z^{\text{soc}} & \mathbf{U}_x^{\text{soc}} - i\mathbf{U}_y^{\text{soc}} \\ \mathbf{U}_x^{\text{soc}} + i\mathbf{U}_y^{\text{soc}} & -\mathbf{U}_z^{\text{soc}} \end{bmatrix}. \quad (\text{S30})$$

The wave function of the lowest Landau band has the form  $(0, |0\rangle, 0, |0\rangle)^T$ , so the matrix element can be calculated as

$$\begin{aligned} U_{0,0}^{k_z, k'_z} &= \langle 0, k_x, k_z | \begin{bmatrix} 0 \\ -i\sin(\theta/2) \\ 0 \\ \cos(\theta/2) \end{bmatrix}^\dagger \begin{bmatrix} \mathbf{U}_z^{\text{soc}} & \mathbf{U}_x^{\text{soc}} - i\mathbf{U}_y^{\text{soc}} & 0 & 0 \\ \mathbf{U}_x^{\text{soc}} + i\mathbf{U}_y^{\text{soc}} & -\mathbf{U}_z^{\text{soc}} & 0 & 0 \\ 0 & 0 & \mathbf{U}_z^{\text{soc}} & \mathbf{U}_x^{\text{soc}} - i\mathbf{U}_y^{\text{soc}} \\ 0 & 0 & \mathbf{U}_x^{\text{soc}} + i\mathbf{U}_y^{\text{soc}} & -\mathbf{U}_z^{\text{soc}} \end{bmatrix} \begin{bmatrix} 0 \\ -i\sin(\theta'/2) \\ 0 \\ \cos(\theta'/2) \end{bmatrix} | 0, k'_x, k'_z \rangle \\ &= \cos \frac{\theta - \theta'}{2} \langle 0, k_x, k_z | -\mathbf{U}_z^{\text{soc}} | 0, k'_x, k'_z \rangle, \end{aligned} \quad (\text{S31})$$

which indicates that only the  $z$  component survives.

The transport time due to the diagonal spin-orbit scattering can be found as

$$\frac{\hbar}{\tau_{\text{so}, k_F}^\pm} = 2L_z \frac{\Lambda I_S}{\hbar v_F} \sum_{k'_x} |\langle 0, k_x, k_F | \mathbf{U}_z^{\text{soc}} | 0, k'_x, -k_F \rangle|^2, \quad (\text{S32})$$

which is also proportional to  $I_S$ , the same as those in the absence of the spin-orbit scattering. Therefore, the transport time for the diagonal spin-orbit scattering does not change the conclusion when there is no spin-orbit scattering, and can be absorbed in the definition of  $\tau_{k_F}^\pm$  in Eq (S14).

### 2. Transport time for off-diagonal Spin-orbit Scattering

We generalize the spin-orbit scattering to the form with off-diagonal scattering, i.e.,

$$U = \begin{bmatrix} \mathbf{U}_z^{\text{soc}} & \mathbf{U}_x^{\text{soc}} - i\mathbf{U}_y^{\text{soc}} & \hat{W}_1 & \hat{W}_2 \\ \mathbf{U}_x^{\text{soc}} + i\mathbf{U}_y^{\text{soc}} & -\mathbf{U}_z^{\text{soc}} & \hat{W}_2^\dagger & -\hat{W}_1 \\ \hat{W}_1^\dagger & \hat{W}_2 & \mathbf{U}_z^{\text{soc}} & \mathbf{U}_x^{\text{soc}} - i\mathbf{U}_y^{\text{soc}} \\ \hat{W}_2^\dagger & -\hat{W}_1 & \mathbf{U}_x^{\text{soc}} + i\mathbf{U}_y^{\text{soc}} & -\mathbf{U}_z^{\text{soc}} \end{bmatrix}. \quad (\text{S33})$$

The transport time for spin-orbit scattering can be written in the formula

$$\frac{\hbar}{\tau_{\text{so}, k_F}^\pm} = \frac{\hbar}{\tau_{\text{U}, k_F}^\pm} + \frac{\hbar}{\tau_{\text{W}, k_F}^\pm}, \quad (\text{S34})$$

where

$$\frac{\hbar}{\tau_{\text{U}, k_F}^\pm} = 2L_z \frac{\Lambda I_S}{\hbar v_F} \sum_{k'_x} |\langle 0, k_x, k_F | \mathbf{U}_z^{\text{soc}} | 0, k'_x, -k_F \rangle|^2, \quad (\text{S35})$$

$$\frac{\hbar}{\tau_{\text{W}, k_F}^\pm} = L_z \frac{\Lambda(1 - I_S)}{2\hbar v_F} \sum_{k'_x} |\langle 0, k_x, k_F | \hat{W}_1 + \hat{W}_1^\dagger | 0, k'_x, -k_F \rangle|^2. \quad (\text{S36})$$

The off-diagonal part transport time can be calculated by the following process:

$$\begin{aligned}
U_{0,0}^{k_z,k'_z} &= \langle 0, k_x, k_z | \begin{bmatrix} 0 \\ -i\sin(\theta/2) \\ 0 \\ \cos(\theta/2) \end{bmatrix}^\dagger \begin{bmatrix} 0 & 0 & \hat{W}_1 & \hat{W}_2 \\ 0 & 0 & \hat{W}_2^\dagger & -\hat{W}_1 \\ \hat{W}_1^\dagger & \hat{W}_2 & 0 & 0 \\ \hat{W}_2^\dagger & -\hat{W}_1^\dagger & 0 & 0 \end{bmatrix} \begin{bmatrix} 0 \\ -i\sin(\theta'/2) \\ 0 \\ \cos(\theta'/2) \end{bmatrix} | 0, k'_x, k'_z \rangle \\
&= -i \sin \frac{\theta}{2} \cos \frac{\theta'}{2} \langle 0, k_x, k_z | \hat{W}_1 | 0, k'_x, k'_z \rangle + i \sin \frac{\theta'}{2} \cos \frac{\theta}{2} \langle 0, k_x, k_z | \hat{W}_1^\dagger | 0, k'_x, k'_z \rangle,
\end{aligned} \tag{S37}$$

$$U_{0,0}^{k_F,-k_F} = -i \sin \frac{\theta}{2} \cos \frac{\theta}{2} \langle 0, k_x, k_F | \hat{W}_1 + \hat{W}_1^\dagger | 0, k'_x, -k_F \rangle, \tag{S38}$$

$$\begin{aligned}
\frac{\hbar}{\tau_{W,k_F}^\pm} &= 2L_z \frac{\Lambda}{\hbar v_F} \sin^2 \frac{\theta}{2} \cos^2 \frac{\theta}{2} \sum_{k'_x} |\langle 0, k_x, k_F | \hat{W}_1 + \hat{W}_1^\dagger | 0, k'_x, -k_F \rangle|^2 \\
&= L_z \frac{\Lambda}{2\hbar v_F} \sin^2 \theta \sum_{k'_x} |\langle 0, k_x, k_F | \hat{W}_1 + \hat{W}_1^\dagger | 0, k'_x, -k_F \rangle|^2 \\
&= L_z \frac{\Lambda(1-I_S)}{2\hbar v_F} \sum_{k'_x} |\langle 0, k_x, k_F | \hat{W}_1 + \hat{W}_1^\dagger | 0, k'_x, -k_F \rangle|^2.
\end{aligned} \tag{S39}$$

### 3. Total transport time and the resistivity

The total transport time is given by the summation of those from all the scattering mechanisms, i.e., the spin-independent scattering and spin-orbit scattering in our case

$$\begin{aligned}
\frac{\hbar}{\tau_{\text{total}}^\pm} &= \frac{\hbar}{\tau_{\text{scaler},k_F}^\pm} + \frac{\hbar}{\tau_{U,k_F}^\pm} + \frac{\hbar}{\tau_{W,k_F}^\pm} \\
&= 2L_z \frac{\Lambda I_S}{\hbar v_F} \sum_{k'_x} |\langle 0, k_x, k_F | U(\mathbf{r}) | 0, k'_x, -k_F \rangle|^2 \\
&\quad + 2L_z \frac{\Lambda I_S}{\hbar v_F} \sum_{k'_x} |\langle 0, k_x, k_F | U_z^{\text{soc}} | 0, k'_x, -k_F \rangle|^2 \\
&\quad + L_z \frac{\Lambda(1-I_S)}{2\hbar v_F} \sum_{k'_x} |\langle 0, k_x, k_F | \hat{W}_1 + \hat{W}_1^\dagger | 0, k'_x, -k_F \rangle|^2.
\end{aligned} \tag{S40}$$

According to Eqs. (S40), both the spin-independent part  $1/\tau_{\text{scaler},k_F}^\pm$  and the diagonal spin-orbit scattering part  $1/\tau_{U,k_F}^\pm$  are proportional to  $I_S$  but the off-diagonal spin-orbit scattering part  $1/\tau_{W,k_F}^\pm$  is proportional to  $(1-I_S)$ . We assume that

$$\sum_{k'_x} |\langle 0, k_x, k_F | U_z^{\text{soc}} | 0, k'_x, -k_F \rangle|^2 \propto \sum_{k'_x} |\langle 0, k_x, k_F | U(\mathbf{r}) | 0, k'_x, -k_F \rangle|^2, \tag{S41}$$

So we have  $1/\tau_{U,k_F}^\pm \propto 1/\tau_{\text{scaler},k_F}^\pm$ .

For the off-diagonal spin-orbit scattering part, considering the dimension of the operator  $|\mathbf{k} \times \mathbf{k}'|^2$ , we assume that

$$\frac{\hbar}{\tau_{W,k_F}^\pm} \propto (1-I_S)B^2. \tag{S42}$$

Using Eq. (S11), we have

$$\begin{aligned}
\rho_{zz} &= \frac{h\pi L_y}{e^2 v_F^0 \Lambda} \left( \int_{-L_y/2\ell_B^2}^{L_y/2\ell_B^2} dk_x \tau_{\text{total}}^{\pm} \right)^{-1} \\
&= \frac{h\pi}{e^3 v_F^0 \Lambda B} \frac{\hbar}{\tau_{\text{total}}^{\pm}} \\
&= \frac{h\pi}{e^3 v_F^0 \Lambda B} \left( \frac{\hbar}{\tau_{\text{scaler}, k_F}^{\pm}} + \frac{\hbar}{\tau_{\text{U}, k_F}^{\pm}} + \frac{\hbar}{\tau_{\text{W}, k_F}^{\pm}} \right) \\
&= \frac{h\pi}{e^3 v_F^0 \Lambda B} \left[ \alpha_1 \frac{I_S}{B} + \alpha_2 (1 - I_S) B^2 \right], \tag{S43}
\end{aligned}$$

where the  $\alpha_1$  term is due to the spin-independent scattering and diagonal spin-orbit scattering and the  $\alpha_2$  term is due to the off-diagonal spin-orbit scattering. By adjusting the ratio  $\alpha_1/\alpha_2$ , we can have a better fitting to the experimental data.

#### 4. Definition of magnetoresistance

In Fig. 1(d), the magnetoresistance is defined as

$$\text{MR} = \frac{\rho_{zz}(B) - \rho_{zz}(B_0)}{\rho_{zz}(B_0)}. \tag{S44}$$

Because our theory works only in the quantum limit,  $B_0$  cannot be 0. The value of  $B_0$  is chosen in the quantum limit. For  $\widetilde{M}_\perp M_z < 0$  (the non-trivial case),  $B_0 = 8$  Tesla, because the resistance is roughly the same at 0 T and 8 T in Ref. [10]. For  $\widetilde{M}_\perp M_z > 0$  (the trivial case), the magnetoresistance is defined in a way that MR is 50% at 5 Tesla, consistent with Ref. [10].

### C. Scattering matrix elements

To evaluate the module square of the scattering matrix elements under the average of impurity configurations, we need to calculate  $\sum_{i,j} I_{\nu,\mu}(\mathbf{R}_i) I_{\nu',\mu'}^*(\mathbf{R}_j)$ . The sum runs over all impurities. The integrals  $I_{\nu,\mu}(\mathbf{R}_i)$  is defined as

$$\begin{aligned}
I_{\nu,\mu}(\mathbf{R}_i) &= \frac{1}{L_x L_z} \int d\mathbf{r} \varphi_{k_x}^{\nu*}(y) \varphi_{k'_x}^\mu(y) U_i(\mathbf{r} - \mathbf{R}_i) \\
&\quad \times e^{i(k'_x - k_x)x + i(k'_z - k_z)z}, \tag{S45}
\end{aligned}$$

where  $U_i(\mathbf{r} - \mathbf{R}_i)$  denotes the scattering potential of a single impurity at the position  $\mathbf{R}_i$ . The  $\hat{\mathbf{y}}$ -direction wavefunction  $\varphi_{k_x}^\nu(y)$  is given in Eq. (S52). Fourier transform the potential by using

$$U_i(\mathbf{r} - \mathbf{R}_i) = \int \frac{d\mathbf{q}}{(2\pi)^3} U_i(\mathbf{q}) e^{i\mathbf{q} \cdot (\mathbf{r} - \mathbf{R}_i)}, \tag{S46}$$

and then using the formula  $\int_{-\infty}^{\infty} dx e^{ikx} = 2\pi\delta(k)$ ,  $I_{\nu,\mu}$  can be rewritten as

$$\begin{aligned}
I_{\nu,\mu}(\mathbf{R}_i) &= \int \frac{d^3\mathbf{q}}{2\pi L_x L_z} e^{-i\mathbf{q} \cdot \mathbf{R}_i} U_i(\mathbf{q}) \int dy \varphi_{k_x}^{\nu*}(y) \varphi_{k'_x}^\mu(y) \\
&\quad \times e^{iq_y y} \delta(q_x + k'_x - k_x) \delta(q_z + k'_z - k_z). \tag{S47}
\end{aligned}$$

Using Eq. (S47),  $\sum_{i,j} I_{\nu,\mu}(\mathbf{R}_i) I_{\nu',\mu'}^*(\mathbf{R}_j)$  can be written as

$$\begin{aligned}
&\sum_{i,j} I_{\nu,\mu}(\mathbf{R}_i) I_{\nu',\mu'}^*(\mathbf{R}_j) \\
&= \sum_{i,j} \int \frac{d^3\mathbf{q}}{2\pi L_x L_z} e^{-i\mathbf{q} \cdot \mathbf{R}_i} U_i(\mathbf{q}) \delta(q_x + k'_x - k_x) \\
&\quad \times \delta(q_z + k'_z - k_z) \int dy \varphi_{k_x}^{\nu*}(y) \varphi_{k'_x}^\mu(y) e^{iq_y y} \\
&\quad \times \int \frac{d^3\mathbf{q}'}{2\pi L_x L_z} e^{i\mathbf{q}' \cdot \mathbf{R}_j} U_j(\mathbf{q}') \delta(q'_x + k'_x - k_x) \\
&\quad \times \delta(q'_z + k'_z - k_z) \int dy' \varphi_{k_x}^{\nu'}(y') \varphi_{k'_x}^{\mu'*}(y') e^{-iq'_y y'}. \tag{S48}
\end{aligned}$$

Under the average of impurity configurations, we employ the theory of impurity average [11]

$$\begin{aligned}
\langle \sum_{i,j} e^{i\mathbf{q}' \cdot \mathbf{R}_j - i\mathbf{q} \cdot \mathbf{R}_i} U_i(\mathbf{q}) U_j(\mathbf{q}') \rangle &\approx \sum_i U_i^2(\mathbf{q}) \delta_{\mathbf{q}-\mathbf{q}'} \\
&= (2\pi)^3 \langle U^2(\mathbf{q}) \rangle \delta(\mathbf{q} - \mathbf{q}'), \tag{S49}
\end{aligned}$$

where  $\langle U^2(\mathbf{q}) \rangle \equiv \sum_i U_i^2(\mathbf{q})/V$ . Then we can integrate over  $\mathbf{q}'$  to obtain

$$\begin{aligned}
\mathcal{I}_{\nu,\mu}^{\nu',\mu'} &\equiv \langle \sum_{i,j} I_{\nu,\mu}(\mathbf{R}_i) I_{\nu',\mu'}^*(\mathbf{R}_j) \rangle \\
&= \int \frac{d^3\mathbf{q}}{2\pi L_x L_z} \langle U^2(\mathbf{q}) \rangle \delta(q_x + k'_x - k_x) \\
&\quad \times \delta(q_z + k'_z - k_z) \int dy \varphi_{k_x}^{\nu*}(y) \varphi_{k'_x}^\mu(y) e^{iq_y y} \\
&\quad \times \int dy' \varphi_{k_x}^{\nu'}(y') \varphi_{k'_x}^{\mu'*}(y') e^{-iq_y y'}, \tag{S50}
\end{aligned}$$

where we have used  $\delta^2(q_x + k'_x - k_x) = (L_y/2\pi)\delta(q_x + k'_x - k_x)$ ,  $\delta^2(q_z + k'_z - k_z) = (L_z/2\pi)\delta(q_z + k'_z - k_z)$ .

For the eigen state of the 0+ Landau band, the wave function is given by

$$\langle \mathbf{r} | 0, +, k_x, k_z \rangle = \begin{bmatrix} -i \sin(\theta/2) \psi_{0,k_x k_z}(\mathbf{r}) \\ \cos(\theta/2) \psi_{0,k_x k_z}(\mathbf{r}) \end{bmatrix}, \tag{S51}$$

where

$$\begin{aligned}\psi_{\nu,k_x k_z}(\mathbf{r}) &= \frac{e^{ik_x x + ik_z z}}{\sqrt{L_x L_z}} \varphi_{\nu,k_x}(y), \\ \varphi_{\nu,k_x}(y) &= \frac{e^{-(y-y_0)^2/2\ell_B^2}}{\sqrt{\nu! 2^\nu \sqrt{\pi} \ell_B}} \mathcal{H}_\nu\left(\frac{y-y_0}{\ell_B}\right),\end{aligned}\quad (\text{S52})$$

where  $y_0 = k_x \ell_B^2$  is the guiding center and  $\mathcal{H}_\nu$  are the Hermite polynomials.

Using the wavefunctions Eq. (S51), the scattering matrix elements between state  $|0, +, k_x, k_z\rangle$  and state  $|0, +, k'_x, k'_z\rangle$  can be written as

$$\begin{aligned}U_{0,0}^{k_z,k'_z} &\equiv \cos \frac{\theta - \theta'}{2} \langle 0, k_x, k_z | U(\mathbf{r}) | 0, k'_x, k'_z \rangle \\ &= \sum_i I_{0,0}(\mathbf{R}_i).\end{aligned}\quad (\text{S53})$$

and thus  $\langle |U_{0,0}^{k_z,k'_z}|^2 \rangle = \mathcal{I}_{0,0}^{0,0}$ . With  $\nu = 0$  and  $\mu = 0$  in Eq. (S50), we have

$$\begin{aligned}\mathcal{I}_{0,0}^{0,0} &= \int \frac{d^3 \mathbf{q}}{2\pi L_x L_z} \langle U^2(\mathbf{q}) \rangle \delta(q_x + k'_x - k_x) \\ &\quad \times \delta(q_z + k'_z - k_z) \left| \int dy \varphi_{k_x}^{0*}(y) \varphi_{k_x - q_x}^0(y) e^{iq_y y} \right|^2.\end{aligned}\quad (\text{S54})$$

With the wavefunction Eq. (S52), we can find

$$\int dy \varphi_{k_x}^{0*}(y) \varphi_{k_x - q_x}^0(y) e^{iq_y y} = e^{-\ell_B^2(q_\perp^2 - 2iq_x q_y + i4k_x q_y)/4},\quad (\text{S55})$$

and

$$\left| \int dy \varphi_{k_x}^{0*}(y) \varphi_{k_x - q_x}^0(y) e^{iq_y y} \right|^2 = e^{-q_\perp^2 \ell_B^2/2}.\quad (\text{S56})$$

Therefore Eq. (S54) becomes

$$\begin{aligned}\langle |U_{0,0}^{k_z,k'_z}|^2 \rangle &= \cos^2 \frac{\theta - \theta'}{2} \int \frac{d^3 \mathbf{q}}{2\pi L_x L_z} \langle U^2(\mathbf{q}) \rangle e^{-q_\perp^2 \ell_B^2/2} \\ &\quad \times \delta(q_x + k'_x - k_x) \delta(q_z + k'_z - k_z).\end{aligned}\quad (\text{S57})$$

#### D. Numerical scheme for $\Lambda$

A widely used approximation is that

$$\begin{aligned}f &= \int_{-\infty}^{\infty} dx \frac{1/c}{(g(x) - g(x_0))^2 + 1/c^2} \\ &= \int_{-\infty}^{\infty} dx \pi \delta(g(x) - g(x_0)),\end{aligned}\quad (\text{S58})$$

but we correct this approximation with an extra factor  $\Lambda$  [3], so that

$$\begin{aligned}f &= \int_{-\infty}^{\infty} dx \frac{1/c}{(g(x) - g(x_0))^2 + 1/c^2} \\ &= \int_{-\infty}^{\infty} dx \pi \Lambda \delta(g(x) - g(x_0)).\end{aligned}\quad (\text{S59})$$

To numerically calculate  $\Lambda$ , we analytically calculate the right hand side of the equation and integrate the left hand side numerically. So (Consider  $g(x)$  as a even function monotonous at  $(0, +\infty)$ .)

$$\begin{aligned}f &= \pi \Lambda \int_{-\infty}^{\infty} dx \delta(g(x) - g(x_0)) \\ &= \pi \Lambda \int_{-\infty}^{\infty} dx \left[ \frac{\delta(x - x_0)}{\left| \frac{d(g(x))}{dx} \right|_{x=x_0}} + \frac{\delta(x + x_0)}{\left| \frac{d(g(x))}{dx} \right|_{x=-x_0}} \right] \\ &= 2\pi \Lambda / \left| \frac{d(g(x))}{dx} \right|_{x=x_0}.\end{aligned}\quad (\text{S60})$$

For the  $0+$  band, we need to deal with

$$\int_{-\infty}^{+\infty} \frac{\frac{\hbar}{2\tau_{k_F}^\pm}}{(E_F - E_{0+})^2 + (\frac{\hbar}{2\tau_{k_F}^\pm})^2} dk_z = \frac{2\pi\Lambda}{\hbar v_F},\quad (\text{S61})$$

so we can calculate  $\Lambda$  by the following formula

$$\Lambda = \frac{\hbar v_F}{2\pi} \int_{-\infty}^{+\infty} \frac{\frac{\hbar}{2\tau_{k_F}^\pm}}{(E_F - E_{0+})^2 + (\frac{\hbar}{2\tau_{k_F}^\pm})^2} dk_z.\quad (\text{S62})$$

#### S3. $B_c$ FOR THE $\text{Bi}_2\text{Se}_3$ FAMILY

TABLE S1. The estimate of  $B_c \approx M_0 \hbar / e \widetilde{M}_\perp$ , at which the backscattering is forbidden. The values indicate that the resistance dip is not likely to be observed in the  $\text{Bi}_2\text{Se}_3$  family. The Zeeman effect corrects  $M_\perp$  to  $\widetilde{M}_\perp = M_\perp + (g_z^c - g_z^v) \mu_B \hbar / 4e$ . Parameters are from Ref. [12].

|                                             | $\text{Bi}_2\text{Se}_3$ | $\text{Bi}_2\text{Te}_3$ | $\text{Sb}_2\text{Te}_3$ |
|---------------------------------------------|--------------------------|--------------------------|--------------------------|
| $M_0$ (eV)                                  | -0.169                   | -0.269                   | -0.182                   |
| $M_\perp$ (eV. $\text{\AA}^2$ )             | 29.36                    | 177.28                   | 51.30                    |
| $M_z$ (eV. $\text{\AA}^2$ )                 | 3.35                     | 9.25                     | 22.12                    |
| $g_z^c$                                     | 1.67                     | 9.71                     | 10.80                    |
| $g_z^v$                                     | -9.41                    | -168.18                  | -18                      |
| $\widetilde{M}_\perp$ (eV. $\text{\AA}^2$ ) | 39.87                    | 346.05                   | 78.62                    |
| $B_c$ (Tesla)                               | 277                      | 51                       | 152                      |

#### S4. COMPARISON WITH THE EXPERIMENT ON $\text{Pb}_{1-x}\text{Sn}_x\text{Se}$

For the model parameters for  $\text{Pb}_{1-x}\text{Sn}_x\text{Se}$  in Fig. 1, our definitions are different from those in Ref. [10], so we need to establish the relation of the parameters between the two works, by comparing the lowest Landau band energy in our model

$$E_{0+} = C_0 + C_z k_z^2 - \frac{g_+ B_z}{2} + \frac{C_\perp}{\ell_B^2} + \sqrt{m^2 + V_n^2 k_z^2},\quad (\text{S63})$$

with that in Ref. [10]

$$E_{0+} = \sqrt{\left[|\Delta| - \left(\frac{\hbar\tilde{w}}{2} - \frac{\tilde{g}\mu_B B}{2}\right)\right]^2 + (\hbar v_z k_z)^2}. \quad (\text{S64})$$

Specifically,

$$\begin{aligned} m &= M_0 + M_z k_z^2 + M_\perp \frac{e}{\hbar} B + \frac{(g_z^c - g_z^v)\mu_B}{4} B \\ &= -|\Delta| + \left(\frac{\hbar\tilde{w}}{2} - \frac{\tilde{g}\mu_B B}{2}\right), \\ V_n &= \hbar v_z. \end{aligned} \quad (\text{S65})$$

In Ref. [10],  $\tilde{\omega} = eB/\tilde{m}$ , so we have

$$\begin{aligned} M_0 &= -|\Delta| = -0.01 \text{ eV}, \\ M_\perp &= \frac{\hbar^2}{2\tilde{m}} \approx 13.5 \text{ eV}\cdot\text{\AA}^2, \\ M_z &= 0, \end{aligned} \quad (\text{S66})$$

where  $\Delta = -0.01$  eV and  $\tilde{m}$  is about 0.25 electron mass for  $x = 0.19$ ,  $v_z = 5.0 \times 10^5$  m/s for  $x = 0.14$  and  $4.8 \times 10^5$  m/s for  $x = 0.19$ . However, we take  $\widetilde{M}_\perp = 18 \text{ eV}\cdot\text{\AA}^2$  for  $x = 0.19$  and  $\widetilde{M}_\perp = -4 \text{ eV}\cdot\text{\AA}^2$  for  $x = 0.14$  to have a better fitting to the experiment.

To calculate the resistivity  $\rho_{zz}$  in Fig. 1(d), we need to deal with the cases of  $x = 0.14$  and  $x = 0.19$  in the experiment. Our calculation is based on Eq. (S43). For  $x = 0.19$ , in the experiment  $v_z = 4.8 \times 10^5$  m/s and the carriers are electrons with  $n = 6 \times 10^{16}/\text{cm}^3$ , so the Fermi energy crosses the 0+ Landau band. We take  $\alpha_1 = 100 \text{ eV}\cdot\text{T}$  and  $\alpha_2 = 0.0025 \text{ eV}\cdot\text{T}^{-2}$ . For  $x = 0.14$ , in the experiment  $v_z = 5.0 \times 10^5$  m/s and the carriers are holes with  $n = 2 \times 10^{16}/\text{cm}^3$ , so the Fermi energy crosses the 0- Landau band. We take  $\alpha_1 = 500 \text{ eV}\cdot\text{T}$  and  $\alpha_2 = 0.25 \text{ eV}\cdot\text{T}^{-2}$ .

## S5. RESISTIVITY IN THE PRESENCE OF GAUSSIAN SCATTERING POTENTIAL

See Fig. S2.

- 
- [1] S. Datta, *Electronic Transport in Mesoscopic Systems* (Cambridge University Press, 1997).
  - [2] H.-Z. Lu, J. Shi, and S.-Q. Shen, "Competition between weak localization and antilocalization in topological surface states," *Phys. Rev. Lett.* **107**, 076801 (2011).
  - [3] H. Z. Lu, S. B. Zhang, and S. Q. Shen, "High-field magnetoconductivity of topological semimetals with short-range potential," *Phys. Rev. B* **92**, 045203 (2015).
  - [4] S.-B. Zhang, H.-Z. Lu, and S.-Q. Shen, "Linear magnetoconductivity in an intrinsic topological Weyl semimetal," *New J. Phys.* **18**, 053039 (2016).
  - [5] A. A. Abrikosov, "Quantum magnetoresistance," *Phys. Rev. B* **58**, 2788 (1998).
  - [6] P. Goswami, J. H. Pixley, and S. Das Sarma, "Axial anomaly and longitudinal magnetoresistance of a generic three-dimensional metal," *Phys. Rev. B* **92**, 075205 (2015).
  - [7] H. Bruus and K. Flensberg, *Many-Body Quantum Theory in Condensed Matter Physics: An Introduction* (Oxford Graduate Texts, 2004).
  - [8] S. Hikami, A. I. Larkin, and Y. Nagaoka, "Spin-orbit interaction and magnetoresistance in the two dimensional random system," *Progr. Theor. Phys.* **63**, 707 (1980).
  - [9] H.-Z. Lu, W. Yao, D. Xiao, and S.-Q. Shen, "Intervalley scattering and localization behaviors of spin-valley coupled Dirac fermions," *Phys. Rev. Lett.* **110**, 016806 (2013).
  - [10] B. A. Assaf, *et al.*, "Negative longitudinal magnetoresistance from the anomalous  $N = 0$  Landau level in topological materials," *Phys. Rev. Lett.* **119**, 106602 (2017).
  - [11] G. D. Mahan, *Many-Particle Physics* (Plenum Press, 1990).
  - [12] I. A. Nechaev and E. E. Krasovskii, "Relativistic  $\mathbf{k} \cdot \mathbf{p}$  Hamiltonians for centrosymmetric topological insulators from *ab initio* wave functions," *Phys. Rev. B* **94**, 201410 (2016).

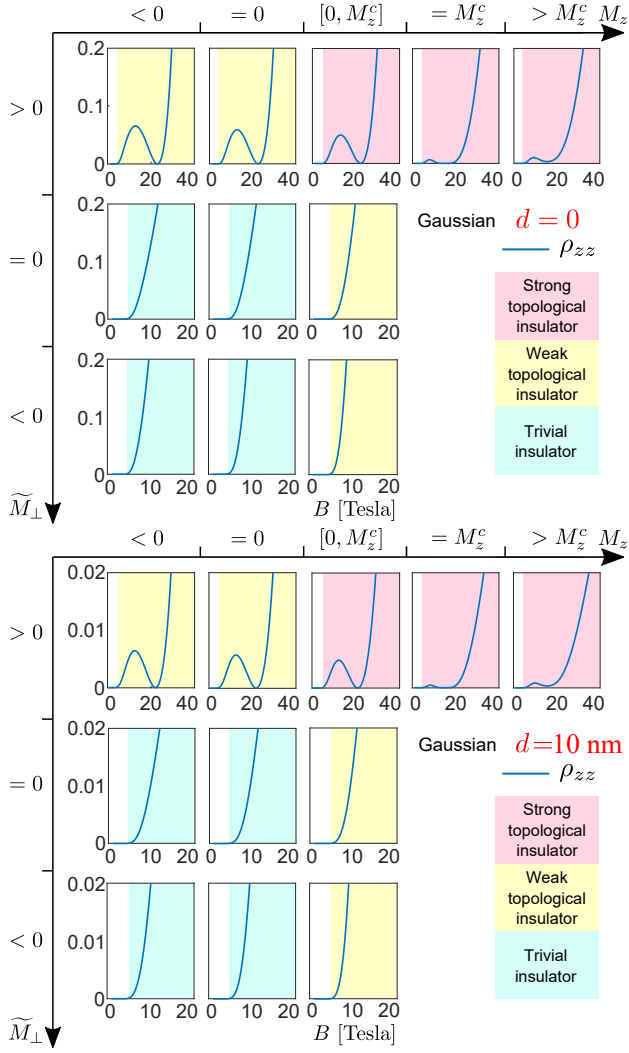

FIG. S2. The same as Fig. 4 of the main text but in the presence of the Gaussian scattering potential ( $d = 0$  and  $d = 10$  nm, in units of  $2\pi\hbar V_{\text{imp}}/e^2$ ).  $d$  is the acting range of the Gaussian potential.
